# Supplementary material for: \~{O}ptimal Dual Vertex Failure Connectivity Labels
Source: arXiv:2208.10168 source file (2022-08-22)
Supplement: Supplementary file 1 [file additional-related-work.tex]

\section{Additional Related Work}\label{sec:add-work}
Our dual-failure vertex connectivity labels are also closely related to \emph{connectivity sensitivity oracles} \cite{DuanConnectivitySODA17,DuanP20}, that provide low-space centralized data-structure for supporting connectivity queries in presence of vertex faults. The main goal in our setting in providing a \emph{distributed} variant of such construction, where each vertex holds only $S(n)/n$ bits of information, where $S(n)$ is the global space of the centralized data-structure. For dual failures, data structures based SPQR trees \cite{BattistaT89} use optimal space of $O(n)$ and report connectivity queries in constant time \cite{BattistaT96}. Duan and Pettie \cite{DuanConnectivitySODA17,DuanP20} provided an ingenues construction that supports multiple vertex faults in nearly optimal space of $\widetilde{O}(n)$. These constructions are built upon highly centralized building blocks, and their distributed implementation is fairly open.

Another seemingly close variant of FT connectivity labels has been studied by Katz, Katz, Korman and Peleg \cite{KatzKKP04}. They provide a labeling scheme, for a given integer $k$, that allows one to report $\min\{k, \kappa(u,v)\}$, where $\kappa(u,v)$ is the vertex-connectivity of a given query pair $u$ and $v$. The state-of-the-art label length for this setting is $O(k \log n)$, due to Hsu and Lu \cite{HsuL09}, which is also tight by \cite{KatzKKP04}. In a very recent work \cite{PettieSTOC22} presented an optimal construction of $k$-vertex connectivity oracles w.r.t space and query time. FT connectivity labels differ from this above mentioned setting.  In our setting, we are also given the labels of the faults $F$, and it is required to determine $u$-$v$ connectivity in $G \setminus F$. This is in particular challenging in cases where a removal of a single vertex disconnects $u$ and $v$, i.e., $\kappa(u,v)=1$. In the latter case, our decoding algorithm is required to return distinct answers for distinct set of faults.
