# Supplementary material for: \~{O}ptimal Dual Vertex Failure Connectivity Labels
Source: arXiv:2208.10168 source file (2022-08-22)
Supplement: Supplementary file 2 [file appendix_new.tex]

\newpage

%\appendix

\section{Single-Source Dual Failure Connectivity Labels}
In this section we design a \emph{single-source} $2$-VFT connectivity labeling scheme with $O(\log^2 n)$-bit labels such that for any target vertex $t$ and any two failed vertices $x,y$, one can (deterministically) determine whether the fixed source $s$ and the target $t$ are $\{x,y\}$-connected using only the labels of $t,x,y$.

\paragraph{Heavy Paths.}
For this part we will need another concept related to the heavy-light decomposition.
Consider the subgraph $T'$ of $T$ formed by taking in all the vertices but only the heavy edges.
The connected components of $T'$ are paths (some of length zero, i.e. isolated vertices), each corresponding to choosing a rooting light vertex in $T$ and going downwards along the heavy edges until reaching a leaf.
Such a path $Q$ is called a \emph{heavy path} of $T$.
We give each heavy path $Q$ a unique ID $\ID(Q)$ of $O(\log n)$ bits (e.g., the ID of its rooting light vertex).
We write $Q_u$ to denote the unique heavy path containing the vertex $u \in V$.
Occasionally, it will be useful to extend a heavy path $Q$ up until the root $s$ of $T$.
We denote this extension by $\overline{Q}$, i.e. $\overline{Q}$ is the unique root-to-leaf path in $T$ containing $Q$.
When traversing in the tree $T$, one can only move between different heavy paths by taking light edges.
Hence Observation \ref{obs:heavy-light} yields:
\begin{observation}
	Any downward path in $T$ intersects only $O(\log n)$ heavy paths.
\end{observation}

\paragraph{Extended IDs Revisited.}
We slightly augment our extended vertex IDs presented in Section \ref{sec:prelim}, by writing in $\EID(u)$ also the number of light vertices in $T[s,u]$, denoted $\nlights(u)$.
That is, the extended ID of vertex $u$ is 
$
\EID(u) = \left[ \ID(u), \AncLabel(u), \ID(\heavy(u)), \AncLabel(\heavy(u)), \nlights(u) \right]
$.
This gives the following:

\begin{lemma}\label{lem:bitstrings}
	Let $v$ be a vertex.
	Assume each $w \in I^{\uparrow} (v)$ is associated with a bit $b(w) \in \{0,1\}$ (which may also depend on $v$).
	For $k = |I^{\uparrow} (v)|$ let $S$ be the $k$-bit string whose $i^{\text{th}}$ bit is $b(w)$, where $w$ is the $i^{\text{th}}$ highest vertex in $I^{\uparrow} (v)$, for all $i$.
	Then, given the string $S$ and $\EID(u)$ of any $u \in I^{\uparrow} (v)$, one can report the bit $b(u)$.
\end{lemma}

\begin{proof}
	There are exactly $\nlights(u)$ vertices higher than $u$ in $I^{\uparrow} (v)$: these are $\parent(w')$ for each light $w' \in T[s,u]$.
	Thus $b(u)$ is the $(\nlights(u) + 1)^\text{th}$ bit of $S$ is $b(u)$.
\end{proof}

\paragraph{Single-Source 1-VFT Labels.}
In Section \ref{sec:single-fault} we presented 2-VFT connectivity labels of size $O(\log^2 n)$.
If we restrict ourselves to \emph{single-source}, we can modify these labels to get $O(\log n)$ size, as follows:

The label of vertex $a$ holds the bitstring composed of $\conn(s, b', \Gsub{b})$ for every $b' \in I(a)$ with $\parent(b') = b$ from highest to lowest, and additionally the bit $\conn(s, \heavy(a), \Gsub{a})$.

When decoding, given the labels of a target $t$ and a failure $x$, we first check if $x$ is a heavy or light ancestor of $t$.
If it is neither, we determine that $s,t$ are $\{x\}$-connected.
If it a heavy ancestor, we report $\conn(s,\heavy(x),\Gsub{x})$ from the label of $x$.
If it is a light ancestor, we report the $(\nlights(x) + 1)^{\text{th}}$ bit of the bitstring part of $t$'s label. (This is essentially using Lemma \ref{lem:bitstrings}.)

To summarize:
\begin{lemma}\label{lem:ss1vft}
	There exists a single-source 1-VFT connectivity labeling with label length $O(\log n)$.
	That it, an $n$-vertex graph $G$ with source vertex $s$ can be preprocessed to compute $O(\log n)$-bit labels such that for any target vertex $t$ and failed vertex $x$, one can (deterministically) determine whether $s$ and $t$ are $\{x\}$-connected.
\end{lemma}

\paragraph{Preliminary Assumptions.}
We make the following structural assumptions throughout:
\begin{itemize}
	\item $x \in T[s,t]$. We always denote by $x'$ the child of $x$ on $T[x,t]$.
	\item $y \notin T[x',t]$. Thus, $x'$ and $t$ are $\{x,y\}$-connected, so it is in fact required to determine the $\{x,y\}$-connectivity of $s$ and $x'$. 
\end{itemize}
These are verified using extended IDs.
If none of $x,y$ is on $T[s,t]$ then we just answer that $s,t$ are $\{x,y\}$-connected.
Otherwise, by swapping $x$ and $y$ if necessary, we may assume that $x$ is the lowest failure on $T[s,t]$, which implies the desired structure.

Additionally, we assume that non of the failures disconnects $s,t$ by itself, as otherwise $s,t$ are clearly $\{x,y\}$-disconnected.
To verify this we use the $1$-VFT labels.
This assumption serves to justify the existence of several detours and related vertices which we define in our labels.
Such explicit justifications are omitted for clarity of presentation.
For the same reason, we also omit explicit explanations about how to extract specific pieces of information from inside a label storing them (e.g. by using Lemma \ref{lem:bitstrings}).

\paragraph{Strategy.}
We will handle differently four different cases based on the location of $y$, where the first three are cases where the failures are dependent, and the last is for independent failures.\footnote{To distinguish between the cases, we use extended IDs.}
\begin{itemize}
	\item The Down case: $y \in T_{x'}$
	\item The Up case: $y \in T[s,x)$
	\item The Side case: $y \in T_x \setminus T_{x'}$
	\item The Independent case: $x$ and $y$ are independent.
\end{itemize}

\subsection{The Down Case: $y \in T_{x'}$}

%\subsubsection*{The Labels:}
%\paragraph{The Labels:}$\quad$\\
%We will need the following definitions. Let $u$ be a vertex.
\paragraph{The Labels:}
Let $u$ be a vertex. Define:
\begin{itemize}
	\item $\alpha_u$: the lowest common ancestor of all vertices $v \in T_u$ with an $s-v$ path internally avoiding $T_u^+$.
	We denote the set of all these vertices $v$ by $A_u$, so $\alpha_u = \LCA(A_u)$.
	
	\item $\beta_u$: the lowest $v \in T[s,\parent(u))$ with a $u-v$ path internally avoiding $T[s,\parent(u)]$. This condition is equivalent to having a path from $T_u$ to $v$ internally avoiding $T[s, \parent(u)]$.
\end{itemize}
The label of vertex $u$ stores the following $O(\log^2 n)$ bits of information:
\begin{itemize}
	\item For every $v' \in I(u)$ with $\parent(v')=v$: 
	\vspace{-\topsep}\begin{itemize}
		\item The vertices $v,v',\alpha_{v'}, \beta_{v'}$.
		\item The bitstring composed of $\conn(s,v',\Gsub{v,w})$ for all $w \in I^{\uparrow} (\alpha_{v'})$ from highest to lowest.
%		\item For every $w \in I^{\uparrow}(\alpha_{v'})$: the bit $\conn(s,v',\Gsub{v,w})$
	\end{itemize}
\end{itemize}

%\subsubsection*{The Decoding Algorithm:}
\paragraph{The Decoding Algorithm:} $\quad$\\
\vspace{-1cm}
\paragraph{Introducing $\alpha_{x'}$.}
As $x' \in I(t) \cup I(x)$, $\alpha_{x'}$ is stored in the label of $t$ or of $x$.
Let $\alpha = \alpha_{x'}$ from now on.
We treat two easy cases:

\noindent{\textit{Case 1: $\alpha_{x'} \notin T_y$.}}
As $\alpha = \LCA(A_{x'})$, there must be some $u \in A_{x'} \setminus T_y$.
Let $P$ be an $s-u$ path internally avoiding $T_{x'}^+$.
Now $P \circ T[u,x']$ certifies that $s,x'$ are $\{x,y\}$-connected.

\noindent{\textit{Case 2: $y \in I^{\uparrow}(\alpha)$.}}
Then $\conn(s,x',\Gsub{x,y})$ is specified along with $\alpha$ and we are done.

From now on, assume that $\alpha \in T_y$ and $y \notin I^{\uparrow}(\alpha)$.
Hence, the child of $y$ on $T[s, \alpha]$ is $\heavy(y)$.
It is not hard to see that $s,\heavy(y)$ are $\{x,y\}$-connected by a path of the form $P \circ T[u,y']$ for some $u \in A_{x'}$, where $P$ internally avoids $T_{x'}^+$.

\paragraph{Introducing $\beta_{\heavy(y)}$.}
We find $\beta_{\heavy(y)}$ in the label of $y$, as $h(y) \in I(y)$.
Let $\beta = \beta_{\heavy(y)}$ from now on.
There are two possible cases.

\noindent{\textit{Case 1: $\beta \in T(x,y)$.}}
Let $P$ be an $\heavy(y)-\beta$ path internally avoiding $T[s,y]$. Then $P \circ T[\beta, x']$ certifies that $\heavy(y),x'$ are $\{x,y\}$-connected, hence this is also true for $s,x'$.

\noindent{\textit{Case 2: $\beta \in T[s,x]$.}}
We prove that $s,x'$ are $\{x,y\}$-disconnected.
Assume the contrary, so $P = P_{s,x',\{x,y\}}$ exists.
Let $\tilde{\alpha}$ be the first vertex from $T_{x'}$ in $P$.
Then $P[s, \tilde{\alpha}]$ internally avoids $T_{x'}^+$, therefore $\tilde{\alpha} \in A_{x'} \subseteq T_{\alpha} \subseteq T_{\heavy(y)} \subseteq T_x$.
Now let $\tilde{\beta}$ be the first vertex from $T[s,y)$ in $P[\tilde{\alpha}, x']$.
\begin{itemize}
	\item If $\tilde{\beta} \in T[s,x)$: Then $T[s,\tilde{\beta}]$ avoids $\{x,y\}$, so as $P$ is a shortest path we obtain $\tilde{\alpha} \in P[s,\tilde{\beta}] = T[s,\tilde{\beta}] \subseteq T[s,x)$. Namely, $\tilde{\alpha}$ is above $x$, which is a contradiction as $\tilde{\alpha} \in T_x$.
	\item Else, $\tilde{\beta} \in T(x,y)$: Then by choice of $\tilde{\beta}$, $P[\tilde{\alpha}, \tilde{\beta}]$ is a path from $T_{\heavy(y)}$ to $\tilde{\beta}$ internally avoiding $T[s,y]$, which contradicts the definition of $\beta = \beta_{\heavy(y)}$ as the lowest such vertex.
\end{itemize}

\paragraph{Reducing Label Size Under Additional Guarantees:}$\quad$\\
If it is guaranteed that $x' = \heavy(x)$ then one can change $I(u)$ to $\{\heavy(u)\}$ in the definition of the labels, and still be able to execute the decoding algorithm. Thus:
\begin{lemma}\label{lem:down_special}
	There are $O(\log n)$-bit labels such that for any $\langle t,x,y\rangle \in V^3$ with $t,y \in T_{\heavy(x)}$ and $y \notin T[\heavy(x), t]$ one can deduce the $\{x,y\}$-connectivity of $s,t$ from the labels of $t,x,y$.
\end{lemma}

\subsection{The Up Case: $y \in T[s,x)$}

\paragraph{The Labels:}
For a vertex $u$ and a heavy path $Q$ ending in leaf $\ell$ such that $u \in \overline{Q}$, define:
\begin{itemize}
	\item $q_u$: the first vertex from $T_u$ in $P_{s,u,\parent(u)}$. Thus, $P_{s,u,\parent(u)} = Q \circ T[q_u, u]$ where $Q$ avoid $T_u$.
	
	\item $a_{u}$: the highest $v \in T[s,\parent(u))$ with an $s-u$ path avoiding $T(v,\parent(u)]$.
	This condition is equivalent to having a $v-u$ path internally avoiding $T[s,\parent(u)]$
	
	\item $b_{u,Q}$: the highest $v \in \overline{Q}(u,\ell]$ with an $s-v$ path internally avoiding $\overline{Q}[u,\ell]$.
	
	\item $c_{u,Q}$: the lowest $v \in \overline{Q}[s,u)$ with a $\succesor(u, Q) - v$ path internally avoiding $\overline{Q}[s,u]$.
\end{itemize}
The label of vertex $u$ stores the following $O(\log^2 n)$ bits of information:
%\begin{itemize}
%	\item For every $v' \in I(u)$ with $\parent(v') = v$:
%	\begin{itemize}
%		\item The vertices $v, v', a_{v'}, q_{v'}, c_{v,Q_v}$ along with $\conn(s,v',\Gsub{v,a_{v'}})$
%		\item For every heavy path $Q$ intersecting $T[s,q_{v'}]$:
%		The vertex $b_{v,Q}$ and $\conn(s,v',\Gsub{v,b_{v,Q}})$
%	\end{itemize}
%\end{itemize}
\begin{itemize}
	\item For every $v' \in I(u)$ with $\parent(v') = v$:
	\vspace{-\topsep}\begin{itemize}
%		\item For every $w \in I^{\uparrow} (v)$: The vertex $w$ and the value $\conn(s, v', \Gsub{v,w})$
		\item The bitstring composed of $\conn(s,v',\Gsub{v,w})$ for all $w \in I^{\uparrow} (v')$ from highest to lowest.
		\item The vertices $v, v', a_{v'}$
		along with $\conn(s,v',\Gsub{v,a_{v'}})$
	\end{itemize}
	\item The vertices $q_{\heavy(y)}$ and $c_{u, Q_u}$.
	\item For every heavy path $Q$ intersecting $T[s, q_{\heavy(u)}]$: $\ID(Q)$, $b_{u, Q}$ and $\conn(s, \heavy(u), \Gsub{u,b_{u,Q}})$.
\end{itemize}

%\subsubsection*{The Decoding Algorithm:}
\paragraph{The Decoding Algorithm:}$\quad$\\
%Denote by $y'$ the child of $y$ on $T[y,x] = \overline{Q_x} [y,x]$.
%Denote by $\ell$ the leaf which is the endpoint of $Q_x$.
We first handle an easy case:

\noindent\textit{Case: $y \in I^{\uparrow} (x)$.}
Then $x' \in I(t) \cup I(x)$, the value $\conn(s,x',\Gsub{x,y})$ is stored in the label of $t$ or of $x$ (to see this set $v = x$, $v' = x'$ and $w = y$), so we are done.

So, from now on we assume $y \notin  I^{\uparrow} (x)$, thus the child of $y$ on $T[y,x]$ is $\heavy(y)$.

\paragraph{Introducing $a_{x'}$.}
As $x' \in I(t) \cup I(x)$, $a_{x'}$ is stored in the label of $t$ or of $x$. Let $a = a_{x'}$ from now on.
We treat two easy cases:

\noindent\textit{Case 1: $a \in T[s,y)$.}
The $s-x'$ path avoiding $T(a, x] \supseteq \{x,y\}$ shows that $s,x'$ are $\{x,y\}$-connected.

\noindent\textit{Case 2: $a=y$.}
Then $\conn(s,x',\Gsub{x,y})$ is specified with $a$.

From now on assume that $a \in T(y,x) = \overline{Q_x} (y,x)$.
Letting $P$ be an $a-x'$ path internally avoiding $T[s,x] \supseteq \{x,y\}$, the path $T[\heavy(y),a_{x'}] \circ P$ now shows that $x',\heavy(y)$ are $\{x,y\}$-connected.

\paragraph{Introducing $q_{\heavy(y)}$.}
The vertex $q_{\heavy(y)}$ is stored in the label of $y$. We treat an easy case.

\noindent\textit{Case: $x \notin T[s,q_{\heavy(y)}]$.}
As $P_{s,q_{\heavy(y)},y} = Q \circ T[s,q_{\heavy(y)}]$ where $Q$ avoids $T_{\heavy(y)} \ni x$, $P_{s,q_{\heavy(y)},y}$ also avoids $x$.
Thus $s,\heavy(y)$ are $\{x,y\}$-connected, hence so are $s,x'$.

From now assume that $x \in T[s,q_{\heavy(y)}]$. Thus $Q_x$ intersects $T[s,q_{\heavy(y)}]$, so $b_{y,Q_x}$ is specified along with $q_{\heavy(y)}$.

\paragraph{Introducing $b_{y,Q_x}$.}
Let $b = b_{y, Q_x}$ from now on. Denote by $\ell$ the leaf which is the endpoint of $Q_x$.
We treat two easy cases:

\noindent\textit{Case 1: $b \in T(y,x) = \overline{Q_x} (y,x)$.}
Letting $P$ be an $s-b$ path $P$ internally avoiding $\overline{Q_x} [y,\ell] \supseteq \{x,y\}$, $P \circ T[b,\heavy(y)]$ shows that $s,\heavy(y)$ are $\{x,y\}$-connected.

\noindent\textit{Case 2: $b = x$.}
Then $\conn(s,\heavy(y),\Gsub{y,x})$ is specified next to $b$.

From now on assume that $b \in \overline{Q_x} (x,\ell]$.

\paragraph{Introducing $c_{x,Q_x}$.}
The vertex $c_{x,Q_x}$ is stored in the label of $x$.
Let $c = c_{x,Q_x}$ from now on.
There are two possible cases:

\noindent\textit{Case 1: $c \in T(y,x) = \overline{Q_x} (y,x)$.}
Let $P$ be a $\succesor(x, Q_x)-c$ path $P$ internally avoiding $\overline{Q_x} [s, x] \supseteq \{x,y\}$.
Let $P'$ be an $s-b$ path internally avoiding $\overline{Q_x} [y,\ell] \supseteq \{x,y\}$.
The concatenation $P' \circ T[b, \succesor(x,Q_x)] \circ P \circ T[c,\heavy(y)]$ now certifies that $s,\heavy(y)$ are $\{x,y\}$-connected.

\noindent\textit{Case 2: $c \in T[s,y] = \overline{Q_x} [s,y]$.}
We prove that $s,x'$ are $\{x,y\}$-disconnected.
Assume the contrary, so $P = P_{s,x',\{x,y\}}$ exists.
We divide to cases:
\begin{itemize}
	\item[(a)] \textit{$P$ avoids $T(y,x) = \overline{Q_x} (y, x)$:}
	Let $\tilde{a}$ be the lowest vertex from $T [s,y)$ appearing in $P$.
	Then $P$ is an $s-x'$ path avoiding $T(\tilde{a}, x]$, and  $\tilde{a}$ is higher than $a$ --- contradicting the definition of $a = a_{x'}$.
	
	\item[(b)] \textit{P avoids $T(x,\ell] = \overline{Q_x} (x, \ell]$:}
	As (a) yields a contradiction, $P$ must hit $\overline{Q_x} (y, x)$.
	Let $\tilde{b}$ be the first vertex from $\overline{Q_x} (y, x)$ in $P$.
	Then $P[s,\tilde{b}]$ is an $s-\tilde{b}$ path internally avoiding $\overline{Q_x} [y, \ell]$, and $\tilde{b}$ is higher than $b$ --- contradicting the definition of $b = b_{y, Q_x}$.
	
	\item[(c)] \textit{$P$ hits  $T(x,\ell] = \overline{Q_x} (x, \ell]$:}
	Again, as (a) yields a contradiction, $P$ must hit $\overline{Q_x} (y, x)$.
	Let $\tilde{c}$ be the first vertex from $\overline{Q_x} (y, x)$ in $P$.
	It cannot be that $P[s,\tilde{c}]$ avoids $\overline{Q_x} (x, \ell]$, as this yields the same contradiction as (b).
	Thus, there is a vertex $u \in \overline{Q_x} (x, \ell]$ that precedes $\tilde{c}$ on $P$.
	As $P$ is a shortest path, it starts by going down along a segment of $T[s,y]$ and never returns to this segment again.
	Therefore, the first vertex from $\overline{Q_x} [s, x]$ that $P[u,\tilde{c}]$ hits is $\tilde{c}$.
	Thus, $\overline{Q_x} [\succesor(x, Q_x), u] \circ P[u, \tilde{c}]$ is a $\succesor(x, Q_x) - \tilde{c}$ path internally avoiding $\overline{Q_x} [s, x]$.
	Also, $\tilde{c}$ is lower than $c$ --- contradicting the definition of $c = c_{x, Q_x}$.
\end{itemize}

\paragraph{Reducing Label Size Under Additional Guarantees:}$\quad$\\
If it is guaranteed that $x' = \heavy(x)$ and $y' = \heavy(y)$, then one can change $I(u)$ to $\{\heavy(u)\}$ in the definition of the labels, and still be able to run the decoding algorithm. Thus:
\begin{lemma}\label{lem:up_special}
	There are $O(\log^2 n)$-bit labels such that for any $\langle t,x,y\rangle \in V^3$ with $t \in T_{\heavy(x)}$ and $x \in T_{\heavy(y)}$ one can deduce the $\{x,y\}$-connectivity of $s,t$ from the labels of $t,x,y$.
\end{lemma}

\subsection{The Side Case: $y \in T_x \setminus T_{x'}$}

%\subsubsection*{The Labels:}
\paragraph{The Labels:}
For a vertex $u$, define:
\begin{itemize}
	\item $g_u$: the last vertex from $T_{\heavy(\parent(u))}$ in  $P_{s,u,\parent(u)}$.
	If this path does not go through $T_{\heavy(\parent(u))}$, we define $g_u = \Null$.
	\item $L_D (u), L_U (u)$: label for Down or Up case with additional guarantees from Lemma \ref{lem:down_special} or Lemma \ref{lem:up_special} respectively.
	\item $L_{SS\text{1F}} (u, G')$: single-source 1-VFT label of $u$ with respect to the subgraph $G' \subseteq G$ with the source $s$ from Lemma \ref{lem:ss1vft}.
\end{itemize}
The label of vertex $u$ stores the following $O(\log^2 n)$ of information:
\begin{itemize}
	\item $L_D (u)$ and $L_U (u)$.
	\item For every $v' \in I(u)$ with $\parent(v') = v$:
	\vspace{-\topsep}\begin{itemize}
		\item $L_{\text{1F}} (u, \Gsub{v})$, $L_{\text{1F}} (v', \Gsub{v})$ and $L_{\text{1F}} (s, \Gsub{v})$.
		\item The vertex $g_{v'}$ with $\conn(s, v', \Gsub{v, g_{v'}})$, $L_D (g_{v'})$ and $L_U (g_{v'})$.
		\item The bitstring composed of  $\conn(s, g_{v'}, \Gsub{v, w})$ for all $w \in I^{\uparrow} (g_{v'})$ from highest to lowest.
	\end{itemize}
\end{itemize}

%\subsubsection*{The Decoding Algorithm:}
\paragraph{The Decoding Algorithm:}$\quad$\\
Let $x''$ be the child of $x$ on $T[x,y]$.
Then $x'' \neq x'$.
If $x''$ is light, then $x'' \in I(y)$, which implies that $L_{\text{1F}} (y, \Gsub{x})$ and $L_{\text{1F}} (s, \Gsub{x})$ are stored in the label of $y$.
As $x' \in I(x) \cup I(t)$, $L_{\text{1F}} (x', \Gsub{x})$ are stored in the label of $x$ or of $t$.
Using these $1$-VFT labels we determine if $s,x'$ are connected in $\Gsub{x} \setminus \{y\} = \Gsub{x,y}$ and we are done.

So, from now on assume $x'' = \heavy(x)$, namely $y \in T_{\heavy(x)}$.

\paragraph{Introducing $g_{x'}$.}
As $x' \in I(x) \cup I(t)$, the vertex $g_{x'}$ is stored in the label of $x$ or of $t$.
Let $g = g_{x'}$ from now on.
If $g = \Null$, then $P_{s,x',x}$ avoids $T_{\heavy(x)} \ni y$, so $s,x'$ are $\{x,y\}$-connected.
If $g = y$, then $\conn(s,x',\Gsub{x,y})$ is stored in the same label, so we are done.

From now on we assume that $g \in V \setminus \{y\}$.
As $g$ is the last vertex from $T_{\heavy(x)} \ni y$ in $P_{s,x',x}$, we have that $x',g$ are $\{x,y\}$-connected.
Thus, it suffices to determine the $\{x,y\}$-connectivity of $s,g$.
Observe that $L_D (g), L_U (g)$ are specified with $g$.
Also, $L_D (x), L_U (x)$ and $L_D (y), L_U (y)$ are stored in the labels of $x,y$.
There are two possible cases:

\noindent\textit{Case 1: $y \notin T[s, g]$.}
Then $g, y \in T_{\heavy(x)}$ and $y \notin T[\heavy(x), g]$. Thus we apply Lemma \ref{lem:down_special} with query $\langle g, x, y \rangle$ to determine the $\{x,y\}$-connectivity of $s,g$.

\noindent\textit{Case 2: $y \in T[s, g)$.}
If $y \in I^{\uparrow} (g)$, then $\conn (s, g, \Gsub{x,y})$ is specified along with $g$ and we are done.
Otherwise, the child of $y$ on $T[s,g]$ is $\heavy(y)$, namely $g \in T_{\heavy(y)}$.
Recall that $y \in T_{\heavy(x)}$.
Thus we apply Lemma \ref{lem:up_special} with query $\langle g, y, x \rangle$ to determine the $\{x,y\}$-connectivity of $s,g$.

\subsection{The Independent Case: $x$ and $y$ are Independent}

%\subsubsection*{The Labels:}
\paragraph{The Labels:}$\quad$\\
We will need the following definitions. Let $u$ be a vertex and $Q$ be a heavy path.
\begin{itemize}
	\item $\ell_{u}$: the last vertex from $T \setminus T_{\parent(u)}$ in $P_{s,u,\parent(u)}$. Thus $P_{s,u,\parent(u)} = T[s, \ell_{u}] \circ Q$ for $Q \subseteq T_u$.
	\item $d_{u,Q}$: the lowest vertex $v \in Q$ with an $s-u$ path internally avoiding $\{u\} \cup (Q \setminus T[s,u))$.
	
\end{itemize}
The label of vertex $u$ consists of the following $O(\log^2 n)$ bits of information:
\begin{itemize}
	\item For every $v' \in I(u)$ with $\parent(v') = v$:	\vspace{-\topsep}\begin{itemize}
		\item The vertices $v,v', \ell_{v'}$.
		\item The bitstring composed of $\conn(s, v', \Gsub{v,w})$ for all $w \in I^{\uparrow}(\ell_{v'})$ from highest to lowest.
	\end{itemize}
	\item For every heavy path $Q$ intersecting $T[s, \ell_{\heavy(u)}]$: $\ID(Q)$ and $d_{u, Q}$.
\end{itemize}

%\subsubsection*{The Decoding Algorithm:}
\paragraph{The Decoding Algorithm:} $\quad$\\
\vspace{-1cm}
\paragraph{Introducing $\ell_{x'}$.}
As $x' \in I(x) \cup I(t)$, $\ell_{x'}$ is stored in the label of $x$ or of $t$. We handle two easy cases:

\noindent\textit{Case 1: $y \notin T[s,\ell_{x'}]$.}
By definition of $\ell_{x'}$, it holds that $P_{s,x',x} = T[s,\ell_{x'}] \circ Q$ where $Q \subseteq T_x$. Therefore, $P_{s,x',x}$ also avoids $y$, so $s,x'$ are $\{x,y\}$-connected.

\noindent\textit{Case 2: $y \in I^{\uparrow} (\ell_{x'})$.}
Then $\conn (s, x', \Gsub{x,y})$ is specified next to $\ell_{x'}$, so we are done.

From now on assume that $y \in T[s,\ell_{x'}]$ and $y \notin I^{\uparrow}(\ell_{x'})$.
Thus, the child of $y$ on $T[s,\ell_{x'}]$ is $\heavy(y)$.
Now $P_{s,x',x} [\heavy(y), x']$ shows that $x'$ and $\heavy(y)$ are $\{x,y\}$-connected.

\paragraph{Introducing $\ell_{\heavy(y)}$.}
%$\quad$\\
%\noindent\textbf{Introducing $\ell_{\heavy(y)}$.}
As $\heavy(y) \in I(y)$, $\ell_{\heavy(y)}$ is stored in the label of $y$.
The cases where $x \notin T[s,\ell_{\heavy(y)}]$ and where $x \in I^{\uparrow} (\ell_{\heavy(y)})$ are treated similarly to the symmetric cases for $\ell_{x'}$. Hence, in these cases we can determine the $\{x,y\}$-connectivity of $s,\heavy(y)$, and thus also of $s,x'$.

From now on assume that $x \in T[s,\ell_{\heavy(y)}]$ and $x \notin I^{\uparrow} (\ell_{\heavy(y)})$.
Thus, the child of $x$ on $T[s,\ell_{\heavy(y)}]$ is $\heavy(x)$.
Now $P_{s,\heavy(y),y}[\heavy(x),\heavy(y)]$ shows that $\heavy(x),\heavy(y)$ are $\{x,y\}$-connected.

\paragraph{Introducing $\ell_{\heavy(x)}$.}
The vertex $\ell_{\heavy(x)}$ is stored in the label of $x$.
We again act in a similar fashion as with $\ell_{\heavy(y)}$.
The only case where we do not finish is when $y \in T[s,\ell_{\heavy(x)}]$ and $y \notin I^{\uparrow} (\ell_{\heavy(x)})$.

\paragraph{Introducing $Q_x$, $Q_y$.}
Let $b_x,b_y$ be the leaves of $T$ which are the endpoints of $Q_x,Q_y$ respectively.
Every $w \in Q_x [\heavy(x), b_x]$ is $\{x,y\}$-connected to $\heavy(x)$, and every $w \in Q_y [\heavy(y), b_y]$ is $\{x,y\}$-connected to $\heavy(y)$.
Let $B = Q_x [\heavy(x), b_x] \cup Q_y [\heavy(y), b_y]$ (i.e., all vertices below $x,y$ in $Q_x, Q_y$ respectively).
Then all vertices in $B$ are $\{x,y\}$-connected, and our goal becomes determining whether there exists $w \in B$ that is $\{x,y\}$-connected to $s$.
We further observe that for $A = T[s,x] \cup T[s,y]$, the path $P_{s,\heavy(y),y} [\heavy(x), \heavy(y)]$ avoids $A$, so by using this path as a bridge between the parts $Q_x [\heavy(x), b_x]$ and $Q_y [\heavy(y), b_y]$ of $B$, we see that all vertices in $B$ are in fact $A$-connected.

\paragraph{Introducing $d_{x,Q_y}$, $d_{y,Q_x}$.}
As $y \in T[s,\ell_{\heavy(x)}]$, $Q_y$ intersects $T[s,\ell_{\heavy(x)}]$, so $d_{x,Q_y}$ is stored in the label of $x$.
We also find $d_{y,Q_x}$ symmetrically.
Denote $d_x = d_{x,Q_y}, d_y = d_{y, Q_x}$.
There are two possible cases:

\noindent\textit{Case 1: $d_x \in B$ or $d_y \in B$.}
Assume $d_x \in B$ ($d_y \in B$ is similar).
Let $P$ be an $s-d_x$ path $P$ internally avoiding $\{x\} \cup (Q_y \setminus T[s,x)) \supseteq \{x,y\}$.
Then $P$ shows that $s$ and $d_x \in B$ are $\{x,y\}$-connected.

\noindent\textit{Case 2: $d_x, d_y \notin B$.}
We prove that all vertices in $B$ are $\{x,y\}$-disconnected to $s$.
Assume the contrary, and let $P$ be an $s-w$ path avoiding $\{x,y\}$ for some $w \in B$.
We may assume that $w$ is the only vertex from $B$ in $P$ (otherwise, replace $w$ by the first hitting point in $B$, and trim $P$ to end there).
Let $u$ be the last vertex from $A$ in $P$.
Assume $u \in T[s,x)$ (the case $u \in T[s,y)$ is similar).
Then $T[s,u] \circ P[u,w]$ internally avoids $\{x\} \cup (Q_y \setminus T[s,x))$.
Now:
\begin{itemize}
	\item If $w \in Q_y [\heavy(y), b_y]$:
	Then $w$ is lower than $d_x$, which contradicts the definition of $d_x = d_{x,Q_y}$.
	\item Else, $w \in Q_x [\heavy(x), b_x]$:
	As all vertices in $B$ are $A$-connected, we may choose a $w-\heavy(y)$ path $P'$ avoiding $A$.
	Let $w'$ be the first vertex from $Q_y$ that $P'$ hits.
	Then $T[s,u] \circ P[u,w] \circ P'[w, w']$ internally avoids $\{x\} \cup (Q_y \setminus T[s,x))$. But as $w' \in Q_y \setminus A$, it is lower than $d_x$, which again contradicts the definition of $d_x$.
\end{itemize}
